# Supplementary material for: Neural Text Sanitization with Privacy Risk Indicators: An Empirical Analysis
Source: arXiv:2310.14312 source file (2023-10-22)
Supplement: Supplementary file 1 [file old_appendix.tex]

\begin{appendices}

\section{Entity-recognizer training parameters}
\label{parameters}

Training parameters for the privacy aware entity recognition model, as described in Section \ref{sec:er}, shown in Table \ref{tbl:Params}.

\begin{table}[h!]
\caption{\label{tbl:Params} Training Parameters for the RoBERTa model}
\begin{tabular}{lcc}  
	\toprule  %\vspace{-1mm}
	 Parameter &  \\
	\midrule 
     Optimizer & AdamW  \\ 
     Learning rate & 2e-5\\ 
     Loss function & CrossEntropy \\
     Inference layer & Linear \\
     Epochs & 3 \\
     Full fine-tuning & yes \\
     GPU & yes \\
     Early stopping & yes \\
	%\bottomrule
\end{tabular}
\end{table}


\section{Label confusion}
\label{label_confusion}

Common semantic type pairs that were found in both datasets to have a high number of difference between the gold label and the label the system assigned to the span (Section \ref{ssec:ld}) are shown in Figure \ref{fig:label_graph}.

\begin{figure}[h!]
\centering
\includegraphics[width = 0.95\textwidth]{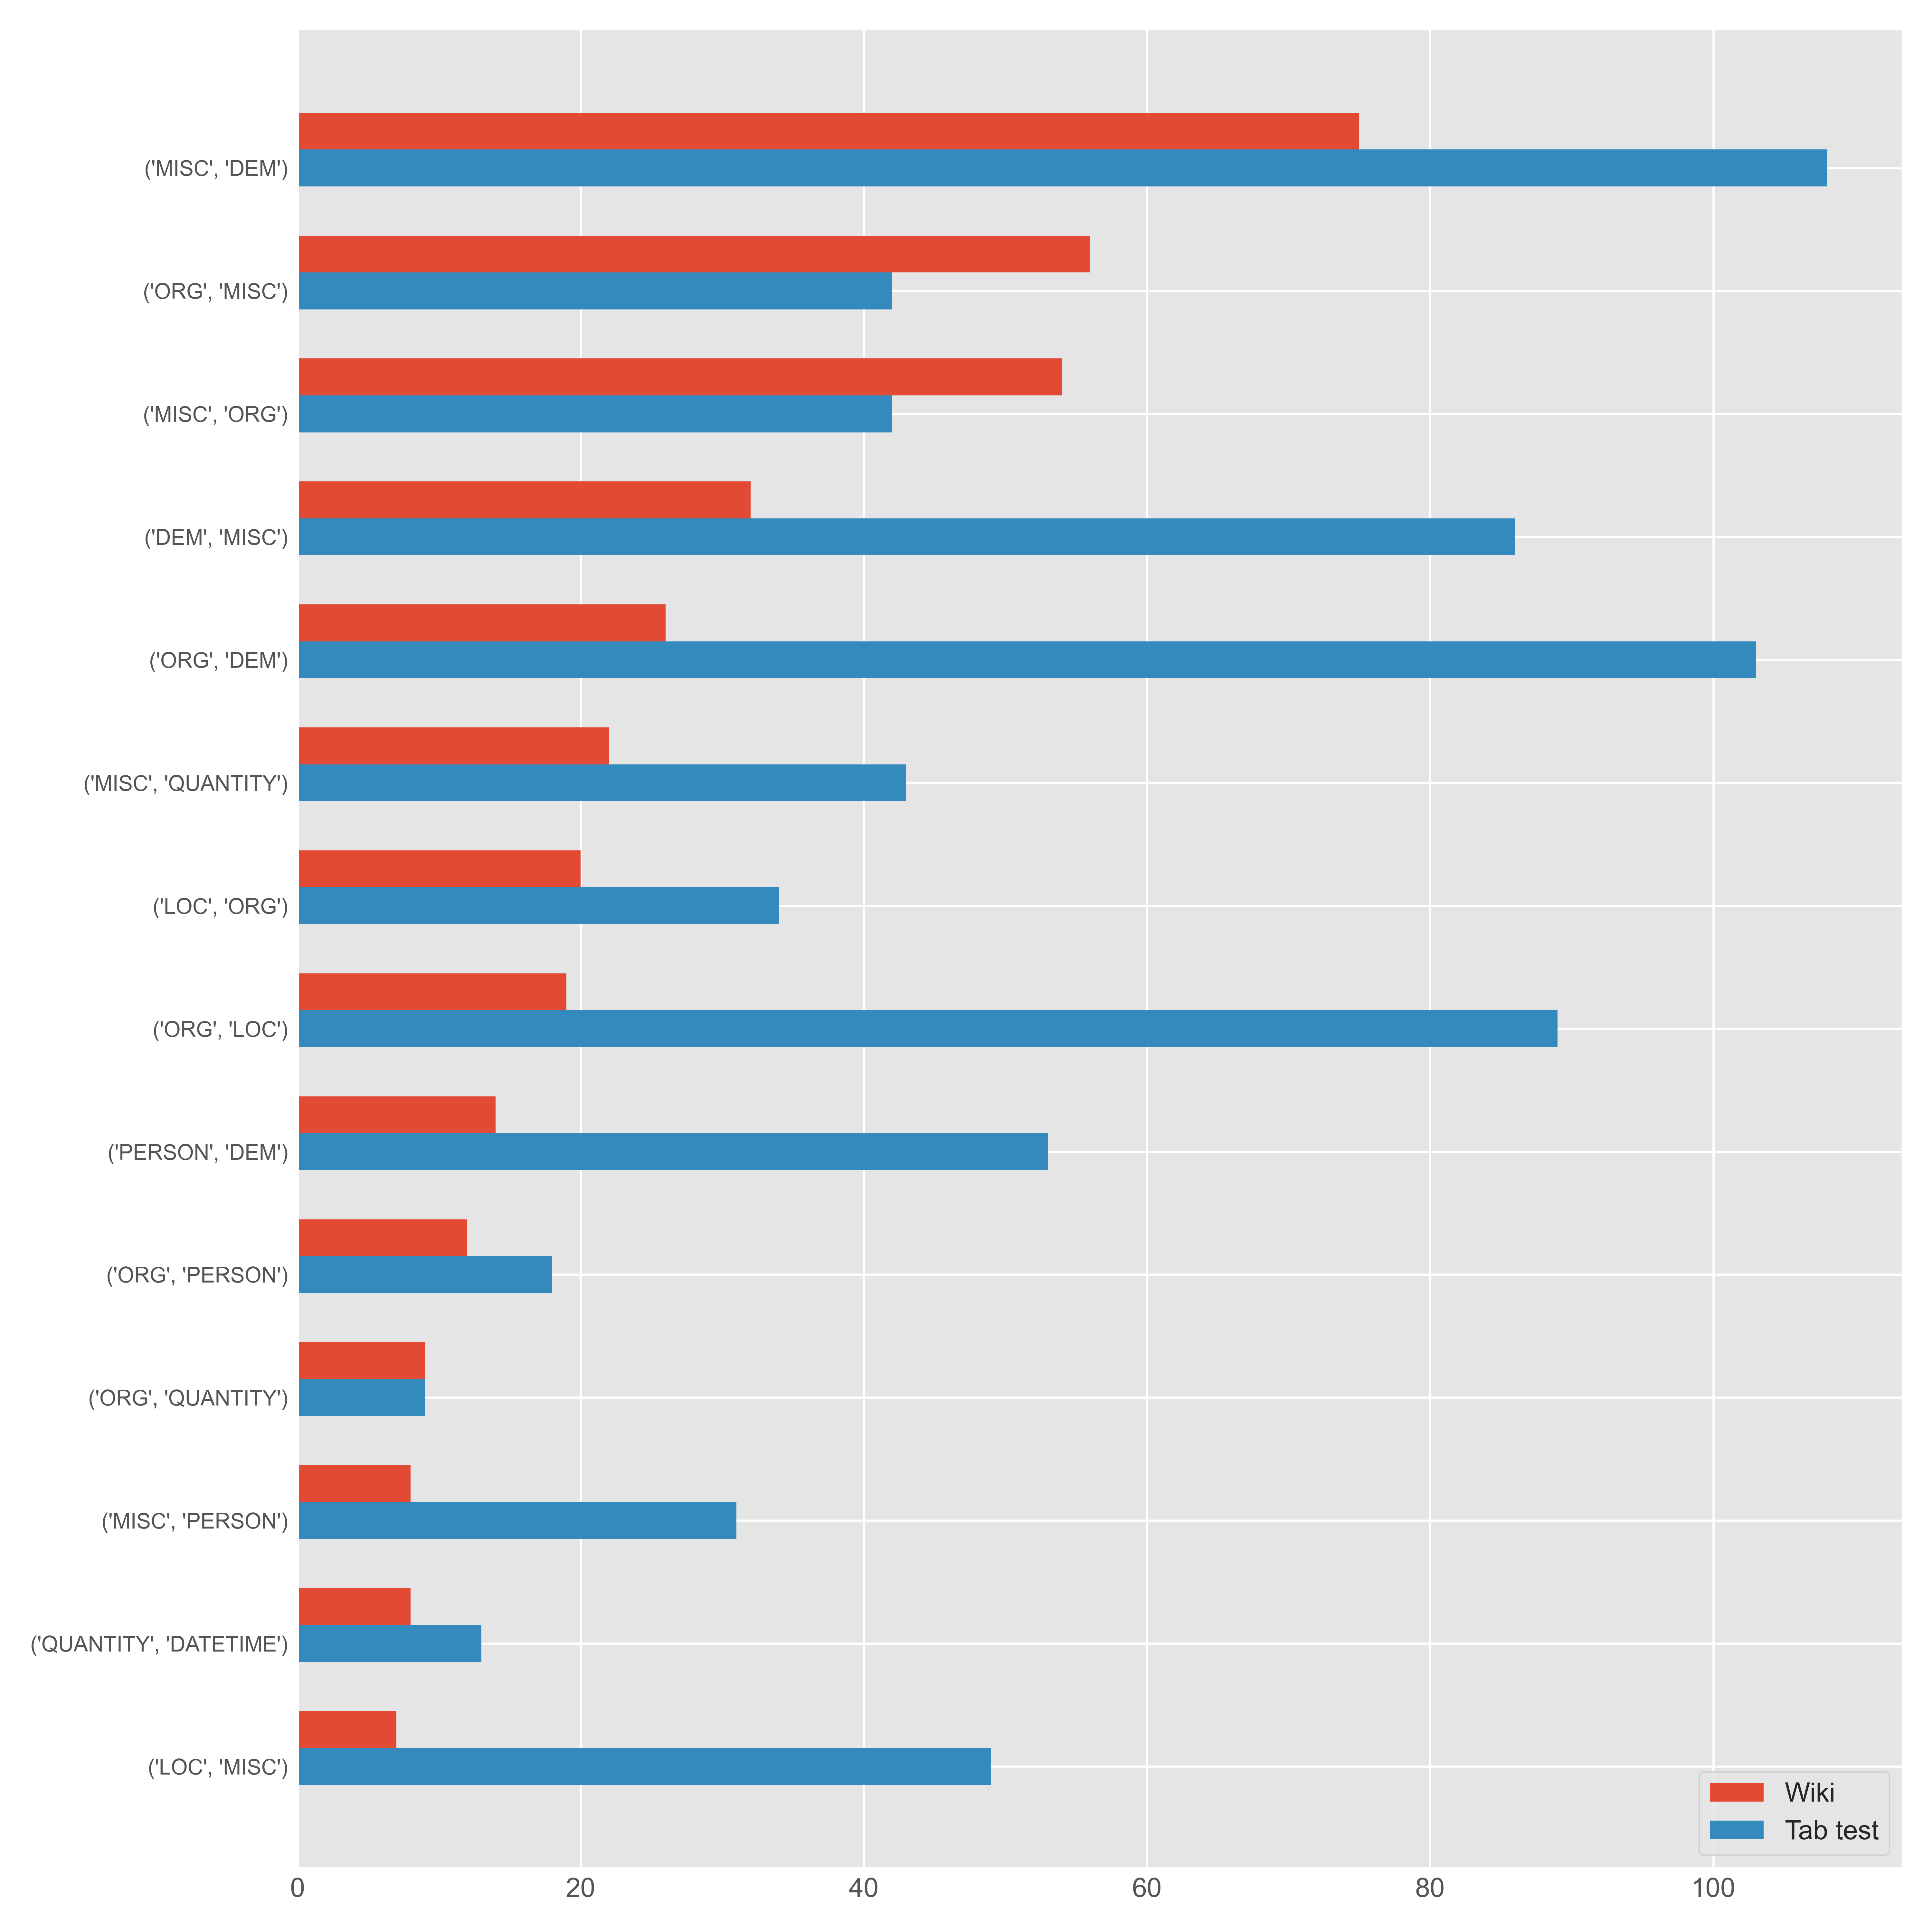}
\caption{Most common label confusion pairs common in the test set of the annotated Wikipedia dataset and the test set of the TAB corpus. The first element of the pair corresponds to the gold standard label, while the second to the label detected by the ER.}
\label{fig:label_graph}
\end{figure}

\section{Autogluon tabular predictor models}
\label{model}

The following Table (Table \ref{tbl:tabular_models}) describes the models the Autogluon tabular predictor employs for the LLM-probability based approach of Section \ref{ssec:tabular}. They are provided here in the order they are trained.

\begin{table}[h!]
\centering
\caption{\label{tbl:tabular_models} Base models of the Tabular predictor in the order they are trained when using the AutoGluon library. Namely, they are trained in this order based on training time and reliability.  This means that more reliable models, like for example random forest based ones, are trained earlier than less reliable ones to ensure efficient training time \cite{autogluon}.}
\begin{tabular}{lcc}  
	\toprule  %\vspace{-1mm}
	 \textbf{Model name} & \textbf{Description}\\
	\midrule 
 \textit{KNeighborsUnif} & k-nearest neighbors classifier with uniform weighting\\
    \textit{KNeighborsDist}& k-nearest neighbors classifier with distance weighting (the inverse of their distance)\\
    \textit{LightGBMXT}& LightGMB model that enables extra trees\\
    \textit{LightGBM}& default light gradient-boosting machine implementation\\
     \textit{RandomForestGini}& random forest classifier with Gini impurity loss function\\
     \textit{RandomForestEntr}& random forest classifier with entropy loss function\\
     \textit{CatBoost}& algorithm that performs gradient boosting on decision trees\\
     \textit{ExtraTreesGini}& extra-trees classifier with Gini impurity loss function\\
     \textit{ExtraTreesEntr}& extra-trees classifier with entropy loss function\\
     \textit{NeuralNetFastAI}& fast AI neural network for classification of tabular data\\
     \textit{XGBoost}& an optimized distributed gradient boosting decision tree model \\
     \textit{LightGBMLarge}& LightGMB model that enables larger models\\
     \textit{NeuralNetTorch}& PyTorch neural network for classification of tabular data\\
     \textit{WeightedEnsemble\_L2}& meta-model that implements Ensemble Selection of the above models\\
	%\bottomrule
\end{tabular}
\end{table}

\section{Training size and performance}
\label{size}

Figure \ref{fig:training_size} shows the $F_1$ score of both Autogluon predictor (LLM probabilities Section \ref{ssec:scrm} and span classification Section \ref{ssec:ppa} respectively) at different training sizes for both datasets. We use a random sample of 1\% to 100\% for each training dataset split.

\begin{figure}[h!]
  \centering
{\includegraphics[width=0.49\textwidth]{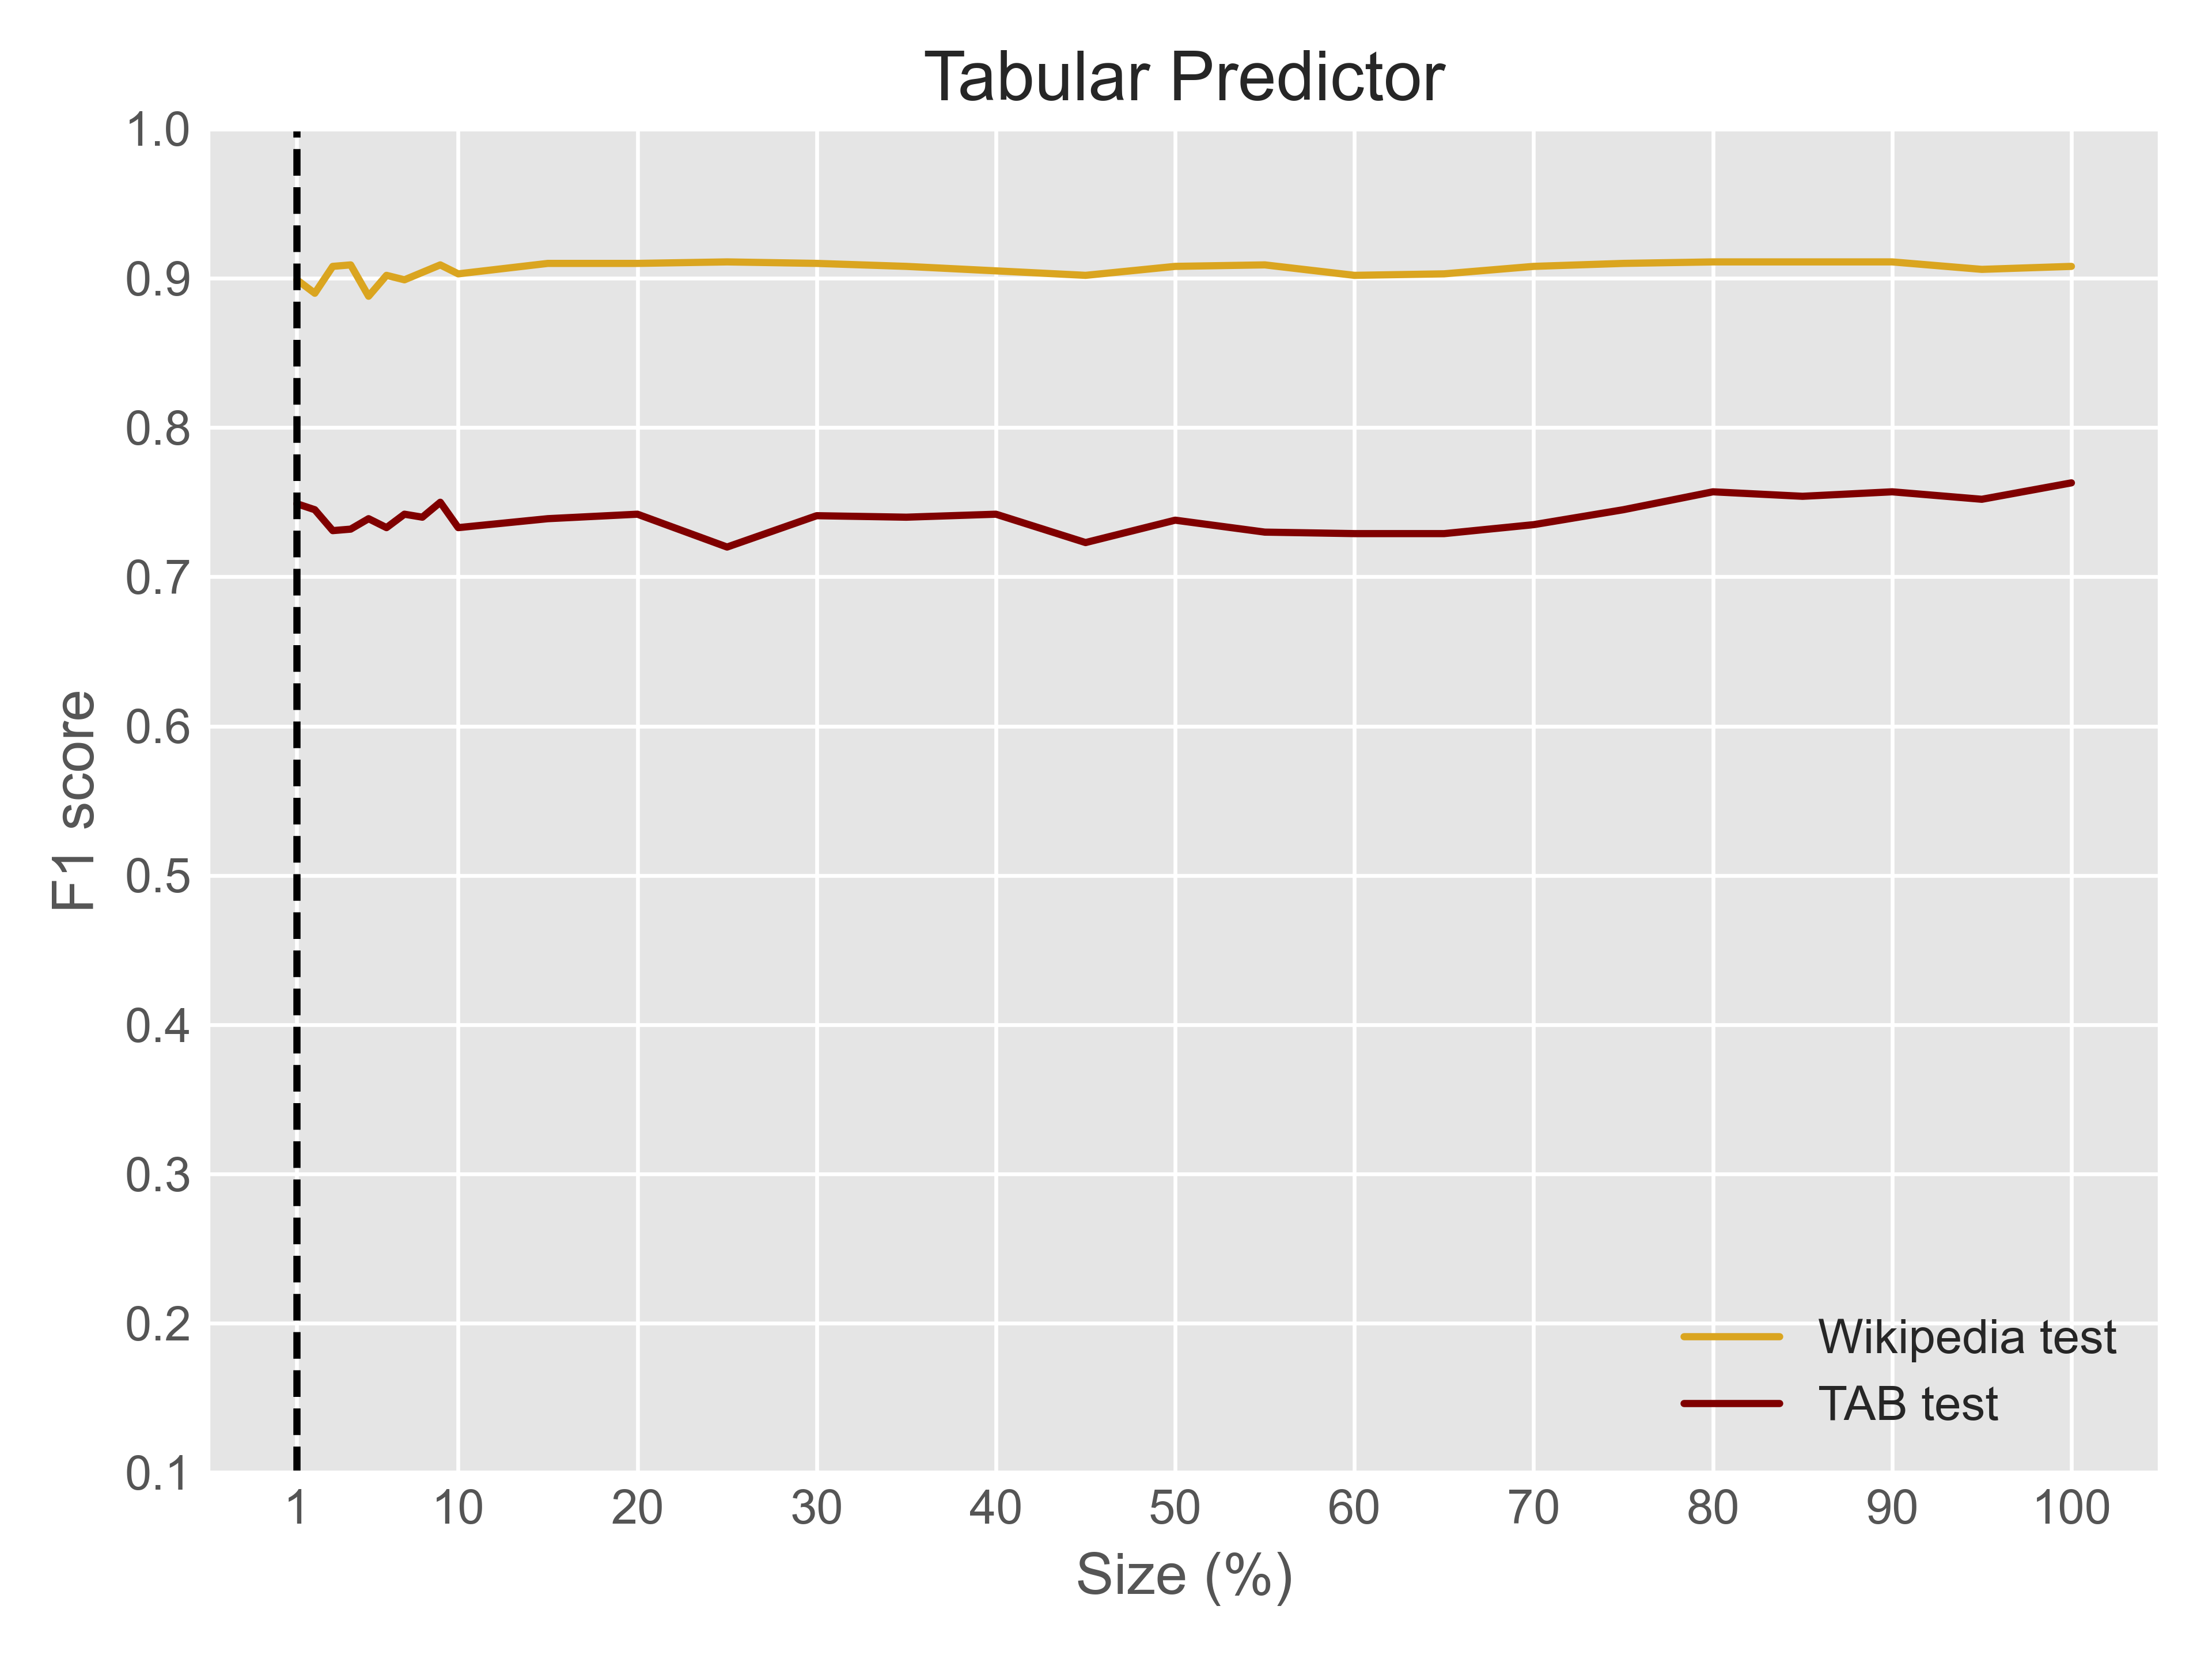}}
  \hfill
{\includegraphics[width=0.49\textwidth]{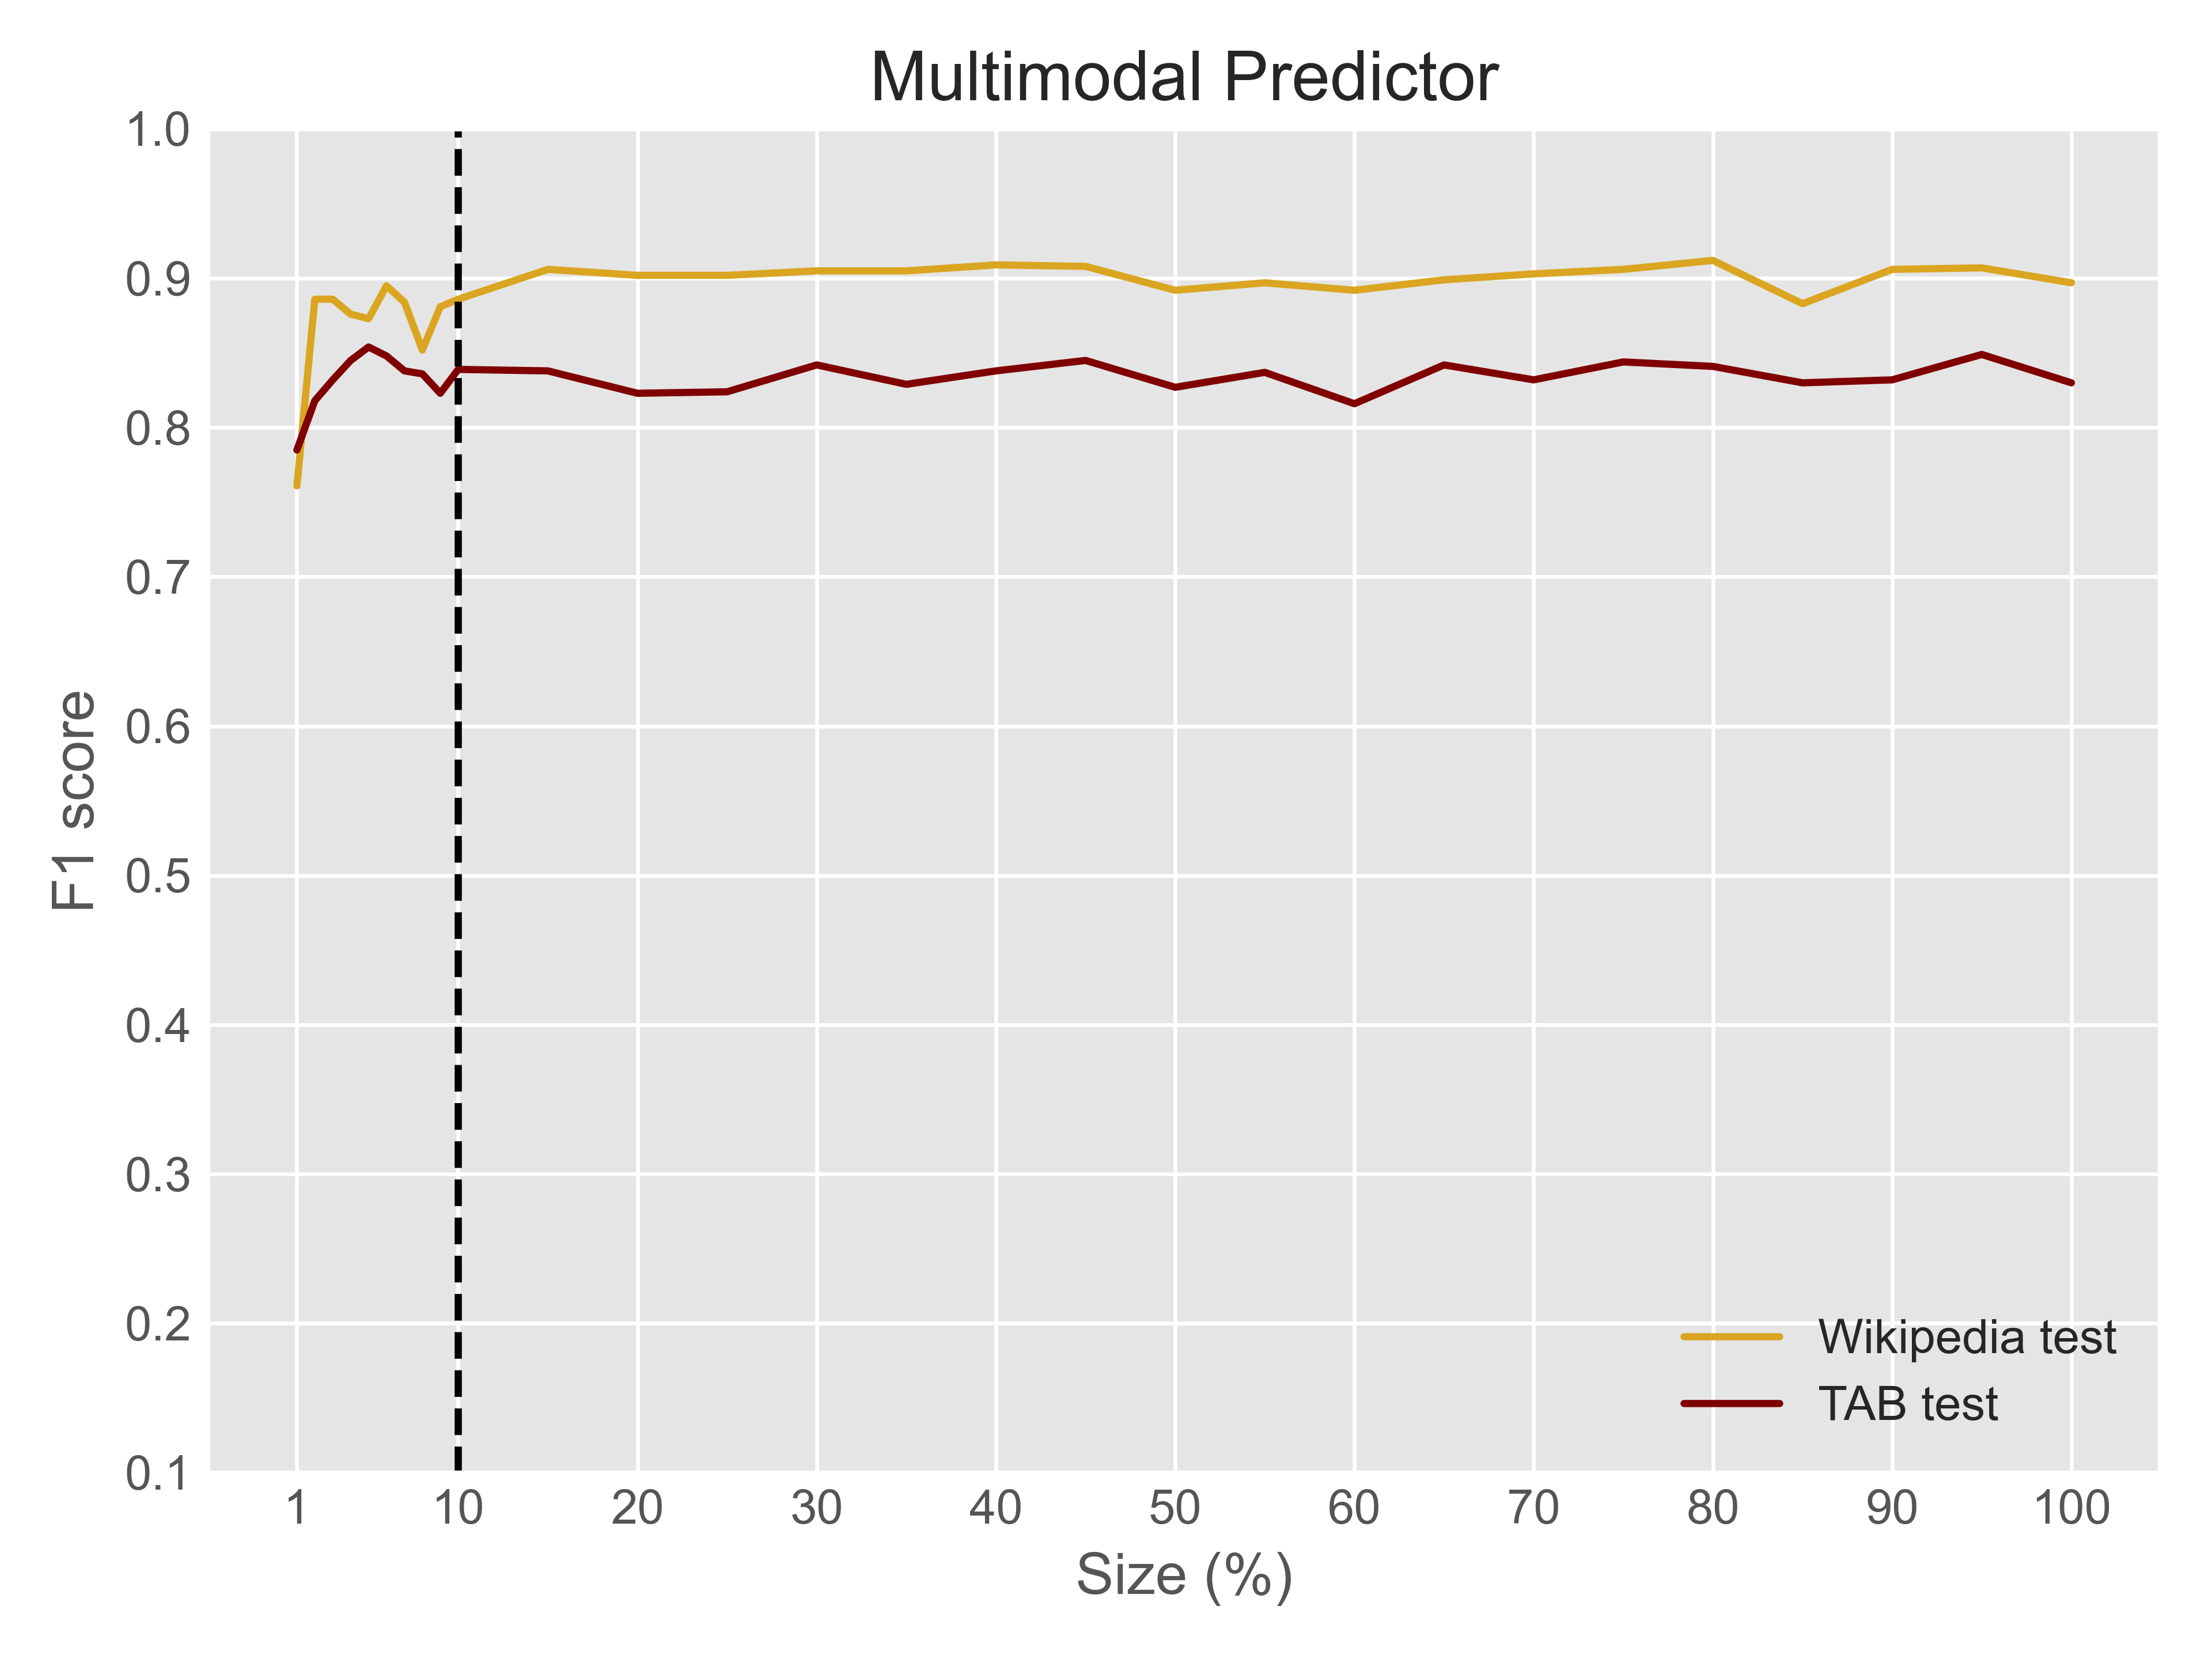}}
  \caption{Performance of the tabular and multimodal predictors when different training sizes are used during training. We report the F1 score for the annotated Wikipedia test dataset and the TAB test dataset as well.}
  \label{fig:training_size}
\end{figure}


\section{Perturbations threshold graphs}
\label{per_graphs}

Figure \ref{fig:perturbation_graph} shows the performance of different perturbation thresholds for both datasets for the training dataset split, with the black line indicating the threshold used in Section \ref{ssec:petrubation} for evaluation.

\begin{figure}[h!]
  \centering
{\includegraphics[width=0.49\textwidth]{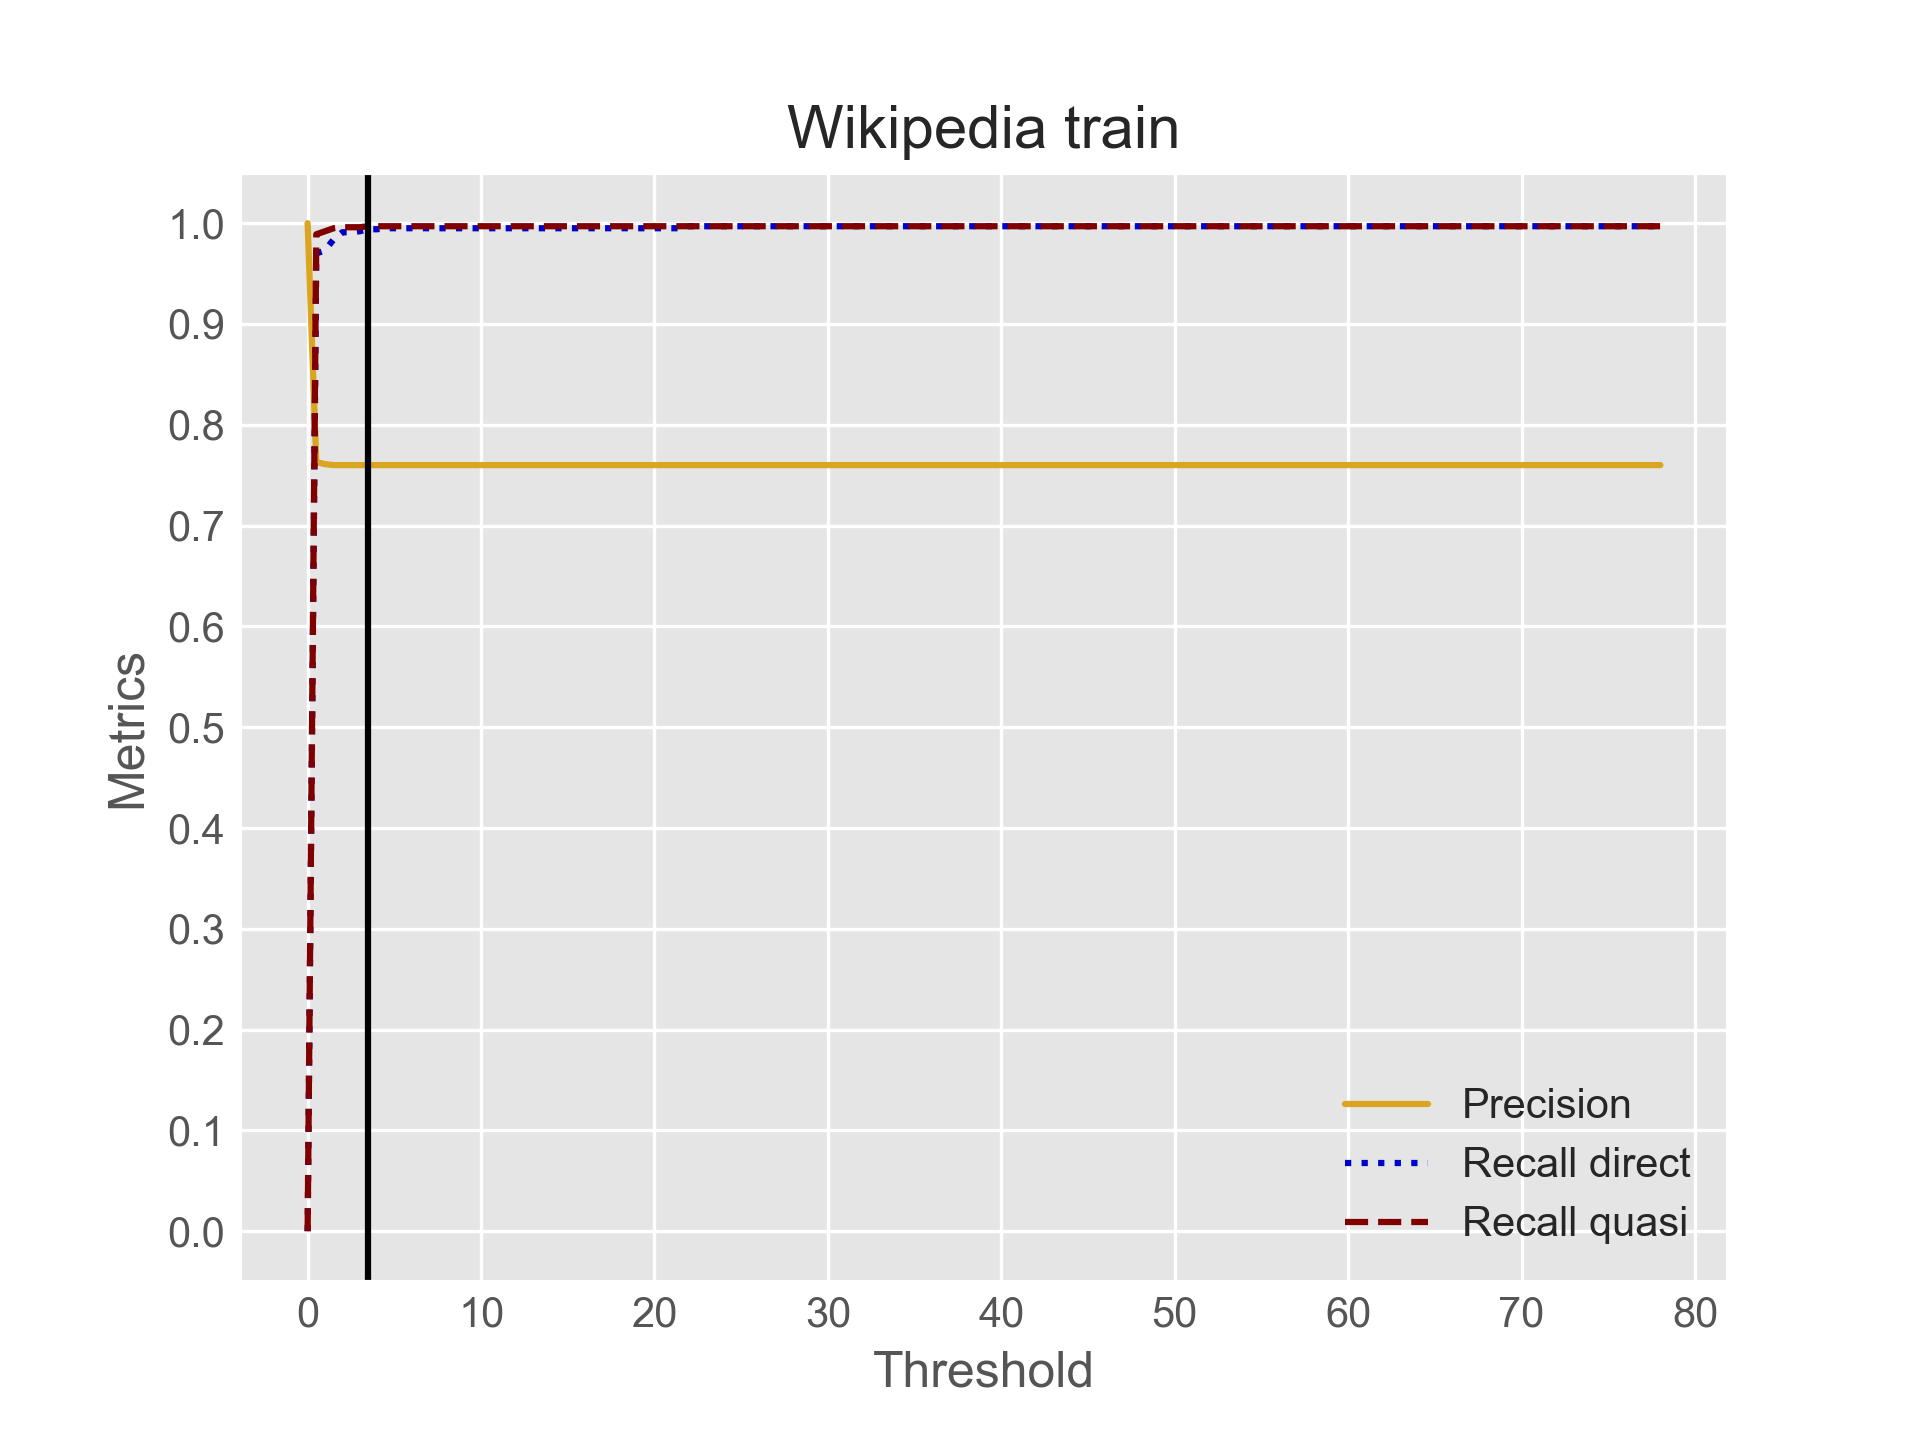}}
  \hfill
{\includegraphics[width=0.49\textwidth]{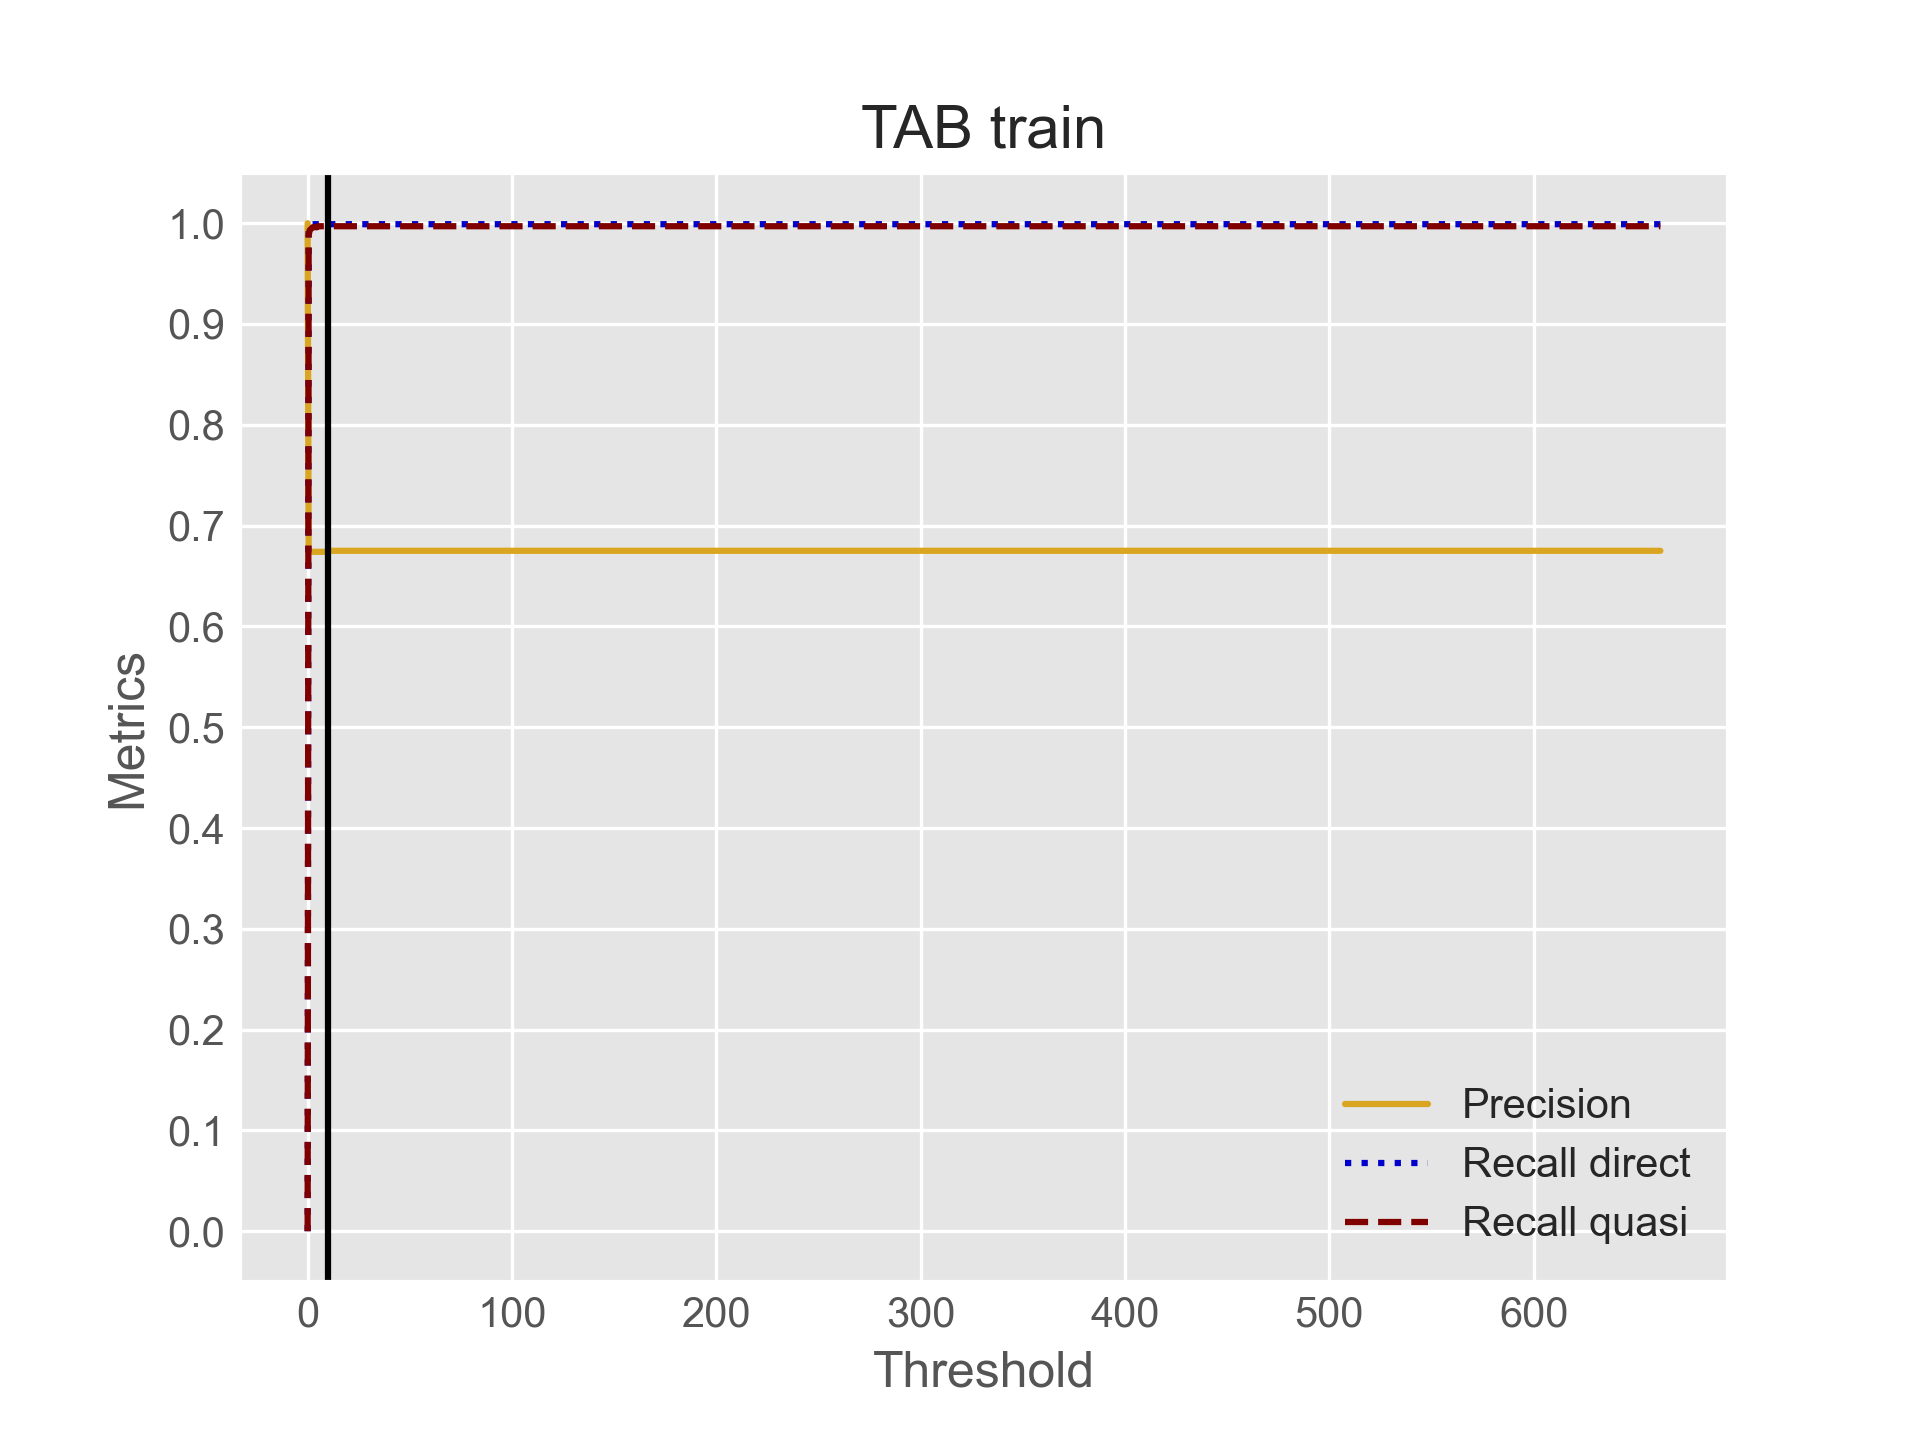}}
  \caption{Precision and recall score for direct and quasi identifiers at different thresholds of probability difference for the Wikipedia and TAB train datasets. The black line indicates the threshold where the cost function is maximized. This is approximately 3.5 for Wikipedia and 10 for TAB)}
  \label{fig:perturbation_graph}
\end{figure}

\section{Human properties from Wikipedia}
\label{human_properties}

The two tables below show the selected Wikidata properties mentioned in Section \ref{sec:properties}:

    \begin{longtable}{|p{2cm}|p{1cm}|p{3cm}|p{6cm}|p{1cm}|}
    \hline
        \textbf{Property} & \textbf{ID} & \textbf{Example} & \textbf{description} & Type \\ \hline
        hairstyle & P8839 & afro & style of cutting, arranging, or combing the hair on the subject's scalp & DEM \\ \hline
        grants & P5460 & Bachelor of Arts & confers degree, honor, award, prize, title, certificate or medal denoting achievement to a person or organization & DEM \\ \hline
        next lower rank & P3729 & General & "lower rank or level in a ranked hierarchy like sport league, military ranks. If there are several possible, list each one and qualify with ""criterion used"" (P1013), avoid using ranks and date qualifiers. For sports leagues/taxa, use specific properties instead." & DEM \\ \hline
        special rank & P5012 & General of the Police of the Russian Federation & non-military rank given to a civil office holder in Russia & DEM \\ \hline
        political ideology & P1142 & social liberalism & political ideology of an organization or person or of a work (such as a newspaper) & DEM \\ \hline
        office held by head of the organization & P2388 & Chief Justice of the United States & position of the head of this item & DEM \\ \hline
        ethnic group & P172 & Ashkenazi Jews & subject's ethnicity (consensus is that a VERY high standard of proof is needed for this field to be used. In general this means 1) the subject claims it themselves, or 2) it is widely agreed on by scholars, or 3) is fictional and portrayed as such) & DEM \\ \hline
        facial hair & P8852 & chin curtain & style of cutting, arranging, or combing the hair on the subject's face (usually on the chin, cheeks, and upper lip region); beard & DEM \\ \hline
        language used & P2936 & Catalan & language widely used (spoken or written) in this place or at this event & DEM \\ \hline
        writing language & P6886 & French & language in which the writer has written their work & DEM \\ \hline
        religion or world view & P8929 & agnosticism & religious or world view affiliation of a person, organization or religious building & DEM \\ \hline
        sex or gender & P21 & male organism & sex or gender identity of human or animal. For human: male, female, non-binary, intersex, transgender female, transgender male, agender. For animal: male organism, female organism. Groups of same gender use subclass of (P279) & DEM \\ \hline
        languages spoken, written or signed & P1412 & Old Chinese & language(s) that a person or a people speaks, writes or signs, including the native language(s) & DEM \\ \hline
        noble title & P97 & baron & titles held by the person & DEM \\ \hline
        position held & P39 & President of the United States & subject currently or formerly holds the object position or public office & DEM \\ \hline
        Y-DNA Haplogroup & P4426 & Haplogroup R1b & Y-DNA haplogroup of a person or organism & DEM \\ \hline
        original language of film or TV show & P364 & italian & "language in which a film or a performance work was originally created. Deprecated for written works and songs; use P407 (""language of work or name"") instead." & DEM \\ \hline
        canonization status & P411 & saint & stage in the process of attaining sainthood per the subject's religious organization & DEM \\ \hline
        occupation & P106 & writer & "occupation of a person; see also ""field of work"" (Property:P101), ""position held"" (Property:P39)" & DEM \\ \hline
        eye color & P1340 & blue-green & color of the irises of a person's eyes & DEM \\ \hline
        culture & P2596 & Inca Empire & human culture or people (or several cultures) associated with this item & DEM \\ \hline
        practiced by & P3095 & cheerleader & type of agents that study this subject or work in this profession & DEM \\ \hline
        official language & P37 & English & language designated as official by this item & DEM \\ \hline
        dialect of & P4913 & Northern Sami & "language of which an item with this property is a dialect. Use in addition to ""subclass of"" (P279) if a languoid is also considered a dialect." & DEM \\ \hline
        political alignment & P1387 & left-wing & political position within the left-right political spectrum & DEM \\ \hline
        educational stage & P7374 & undergraduate education & "educational stage of a specific school; qualifier of ""educated at"" (P69): the education stage of someone's attendance of school" & DEM \\ \hline
        substitute & P2098 & Lieutenant Governor of the United States Virgin Islands & function that serves as deputy/replacement of this function/office (scope/conditions vary depending on office) & DEM \\ \hline
        professorship & P803 & Lucasian Professor of Mathematics & professorship position held by this academic person & DEM \\ \hline
        official religion & P3075 & Islam & official religion in this administrative entity & DEM \\ \hline
        office contested & P541 & Chief Executive of Hong Kong & title of office which election will determine the next holder of & DEM \\ \hline
        sexual orientation & P91 & homosexuality & the sexual orientation of the person -- use IF AND ONLY IF they have stated it themselves, unambiguously, or it has been widely agreed upon by historians after their death & DEM \\ \hline
        kinship to subject & P1039 & daughter-in-law & "qualifier of ""relative"" (P1038) to indicate less usual family relationships (ancestor, son-in-law, adoptions, etc). Indicate how the qualificator item is related to the main item." & DEM \\ \hline
        next higher rank & P3730 & pope & "higher rank or level in a ranked hierarchy like sport league, military ranks. If there are several possible, list each one and qualify with ""criterion used"" (P1013), avoid using ranks and date qualifiers. For sports leagues/taxa, use specific properties instead." & DEM \\ \hline
        academic degree & P512 & Doctor of Philosophy & academic degree that the person holds & DEM \\ \hline
        religion & P140 & Hinduism & religion of a person, organization or religious building, or associated with this subject & DEM \\ \hline
        office held by head of government & P1313 & Prime Minister of the United Kingdom & political office that is fulfilled by the head of the government of this item & DEM \\ \hline
        native language & P103 & Russian & language or languages a person has learned from early childhood & DEM \\ \hline
        members have occupation & P3989 & lawyer & all members of this group share the occupation & DEM \\ \hline
        language of work or name & P407 & Italian & "language associated with this creative work (such as books, shows, songs, or websites) or a name (for persons use ""native language"" (P103) and ""languages spoken, written or signed"" (P1412))" & DEM \\ \hline
        office held by head of state & P1906 & President of Israel & political office that is fulfilled by the head of state of this item & DEM \\ \hline
        military rank & P410 & General & "military rank achieved by a person (should usually have a ""start time"" qualifier), or military rank associated with a position" & DEM \\ \hline
        medical condition & P1050 & spina bifida & any state relevant to the health of an organism, including diseases and positive conditions & DEM \\ \hline
        hair color & P1884 & brown hair & person's hair color. Use P585 as qualifier if there's more than one value & DEM \\ \hline
        title of chess person & P2962 & Grandmaster & title awarded by a chess federation to a person & DEM \\ \hline
    \end{longtable}

    \begin{longtable}{|p{2cm}|p{1cm}|p{3cm}|p{6cm}|p{1cm}|}
        \hline
    \textbf{Property} & \textbf{ID} & \textbf{Example} & \textbf{description} & Type \\ \hline
        classification of race & P2502 & 2015 Schaal Sels & race for which this classification applies & MISC \\ \hline
        contributing factor of & P1537 & critical thinking & thing that is significantly influenced by this cause, but does not directly result from it.  See 'Help:Modeling causes' for examples and discussion. & MISC \\ \hline
        length & P2043 & 15 centimeters & measured dimension of an object & MISC \\ \hline
        conflict & P607 & Battle of Dennewitz & battles, wars or other military engagements in which the person or item participated & MISC \\ \hline
        school of & P1780 & Ain AlBaraha & for a creative work with author with a style influenced by the known author or circle, active in the same period, but a student or follower & MISC \\ \hline
        bowling style & P2545 & Left-arm orthodox spin & type of bowling employed by a cricketer & MISC \\ \hline
        field of training & P8258 & bookselling & profession, position or activity someone learnt during a training, traineeship or apprenticeship & MISC\\ \hline
        used by & P1535 & television watcher & item or concept that makes use of the subject (use sub-properties when appropriate) & MISC \\ \hline
        studied by & P2579 & egyptology & subject is studied by this science or domain & MISC \\ \hline
        hashtag & P2572 & BlackLivesMatter & "hashtag associated with this item. Format: do not include the ""\#"" symbol" & MISC \\ \hline
        worshipped by & P1049 & Zoroastrianism & religion or group/civilization that worships a given deity & MISC \\ \hline
        motto & P1546 & Florebo quocumque ferar & description of the motto of the subject & MISC \\ \hline
        statement is subject of & P805 & death of Osama bin Laden & (qualifying) item that describes the relation identified in this statement & MISC \\ \hline
        GitHub topic & P9100 & bitcoin & GitHub topic for a repository or subject & MISC \\ \hline
        original spelling & P1353 & Aloe steffaniana & original spelling of a scientific name & MISC \\ \hline
        armament & P520 & AIM\-120 AMRAAM & equippable weapon item for the subject & MISC \\ \hline
        architectural style & P149 & French Gothic architecture & architectural style of a structure & MISC \\ \hline
        academic major & P812 & political science & major someone studied at college/university & MISC \\ \hline
        in opposition to & P5004 & Plan Juppé, 1995 & qualifier to indicate the purpose of a social action & MISC \\ \hline
        astronaut mission & P450 & Soyuz TMA-8 & space mission that the subject is or has been a member of (do not include future missions) & MISC \\ \hline
        field of this occupation & P425 & bodyboarding & activity corresponding to this occupation or profession (use only for occupations/professions - for people use Property:P101, for companies use P452) & MISC \\ \hline
        vehicle & P1876 & Soyuz-TMA & vessel involved in this mission, voyage or event & MISC \\ \hline
        test taken & P5021 & SAT & subject took the test or exam, or was assessed per test or method & MISC \\ \hline
        trophy awarded & P4622 & Oscar statuette & trophy awarded at the end of a selection process or of a competition, usually to winners or finishers under the form of a cup, a medal, a diploma & MISC \\ \hline
        sport number & P1618 & 27 & number worn on a player's (competitor's) uniform, equipment, etc & MISC \\ \hline
        Twitter username & P2002 & NASA & this item's username on Twitter; do not include the ??? symbol & MISC \\ \hline
        programming language & P277 & C++ & the programming language(s) in which the software is developed & MISC \\ \hline
        advertises & P6291 & Michelin & cause, organization or product targeted by the advertising campaign, character, jingle or slogan & MISC \\ \hline
        uses & P2283 & paintbrush & item or concept used by the subject or in the operation (see also instrument [P1303] and armament [P520]) & MISC \\ \hline
        study or design for & P6606 & Birds and Irises & finished work of art for which the subject is a preliminary study, design, or conceptual drawing & MISC \\ \hline
        manner of death & P1196 & capital punishment & general circumstances of a person's death; e.g. natural causes, accident, suicide, homicide, etc.  Use 'cause of death' (P509) for the specific physiological mechanism, e.g. heart attack, trauma, pneumonia... & MISC \\ \hline
        evaluation of & P5134 & heart rate & the subject finding is an evaluation or interpretation of the object attribute or test & MISC \\ \hline
        Eight Banner register & P470 & Manchu Bordered Yellow Banner & Manchu household register for people of the Qing Dynasty & MISC \\ \hline
        title of broader work & P6333 & Revue des Deux Mondes & "title of website, journal or other work in which an article (or other publication) is published in. Use ""published in"" (P1433) instead if possible." & MISC \\ \hline
        genre & P136 & war film & creative work's genre or an artist's field of work (P101). Use main subject (P921) to relate creative works to their topic & MISC \\ \hline
        applies to jurisdiction & P1001 & Eurozone & the item (institution, law, public office, public register...) or statement belongs to or has power over or applies to the value (a territorial jurisdiction: a country, state, municipality, ...) & MISC \\ \hline
        playing hand & P741 & left-handedness & hand used to play a racket sport & MISC \\ \hline
        fictional analog of & P1074 & spacecraft & used to link an entity or class of entities appearing in a creative work with the analogous entity or class of entities in the real world & MISC \\ \hline
        inscription & P1684 & O U O S V A V V & inscriptions, markings and signatures on an object & MISC \\ \hline
        broader concept & P4900 & hat & qualifier to indicate a broader concept that the present item is part of, as mapped by an external source. The statement being qualified should be an exact match. & MISC \\ \hline
        legal citation of this text & P1031 & 384 U.S. 436 & legal citation of legislation or a court decision & MISC \\ \hline
        exhibition history & P608 & Saint Anne, Leonardo da Vinci ultimate masterpiece & exhibitions where the item is or was displayed & MISC \\ \hline
        form of creative work & P7937 & novel & structure of a creative work, type of music release & MISC \\ \hline
        has edition or translation & P747 & Orgoglio e pregiudizio & link to an edition of this item & MISC \\ \hline
        nominated for & P1411 & BRIT Awards & "award nomination received by a person, organisation or creative work (inspired from ""award received"" (Property:P166))" & MISC \\ \hline
        voice type & P412 & lyric spinto tenor & person's voice type. expected values: soprano, mezzo-soprano, contralto, countertenor, tenor, baritone, bass (and derivatives) & MISC \\ \hline
        platform & P400 & Xbox 360 & platform for which a work was developed or released, or the specific platform version of a software product & MISC \\ \hline
        drug used for treatment & P2176 & dabrafenib & drug, procedure, or therapy that can be used to treat a medical condition & MISC \\ \hline
        owner of & P1830 & SPY Records & entities owned by the subject & MISC \\ \hline
        fabrication method & P2079 & sericulture & method, process or technique used to grow, cook, weave, build, assemble, manufacture the item & MISC \\ \hline
        connects with & P2789 & Rokin & item with which the item is physically connected & MISC \\ \hline
        totem & P2831 & Siluriformes & in many indigenous cultures an individual or group has a particular totem (e.g. a type of animal) & MISC \\ \hline
        field of work & P101 & linguistic purism & specialization of a person or organization; see P106 for the occupation & MISC \\ \hline
        definition domain & P1568 & set of real numbers & "set of ""input"" or argument values for which a mathematical function is defined" & MISC \\ \hline
        parliamentary term & P2937 & 13th legislature of the Fifth French Republic & term of a parliament or any deliberative assembly & MISC \\ \hline
        exonerated of & P7781 & murder & crime of which the subject was found not to be guilty after having previously been found guilty by a court for that crime & MISC \\ \hline
        carries scientific instrument & P1202 & Astro & scientific instruments carried by a vessel, satellite, or device that are not required for propelling or navigating & MISC \\ \hline
        distribution format & P437 & Blu-ray Disc & method (or type) of distribution for the subject & MISC \\ \hline
        use & P366 & source of information & main use of the subject (includes current and former usage) & MISC \\ \hline
        end cause & P1534 & resignation & qualifier to use together with the end date qualifier (P582) to specify the cause & MISC \\ \hline
        source of income & P2770 & donation & source of income of an organization or person & MISC \\ \hline
        participant in & P1344 & 1992 Winter Olympics & event in which a person or organization was/is a participant; inverse of P710 or P1923 & MISC \\ \hline
        depicted by & P1299 & Traveler Over The Mist Sea & object depicting this subject (creative works, books of the bible) & MISC \\ \hline
        member of the crew of & P5096 & Titanic & person who has been a member of a crew associated with the vessel or spacecraft. For spacecraft, inverse of crew member (P1029), backup or reserve team or crew (P3015) & MISC \\ \hline
        victory & P2522 & 2015 Internationale Wielertrofee Jong Maar Moedig & competition or event won by the subject & MISC \\ \hline
        elected in & P2715 & 1999 German presidential election & qualifier for statements in position held to link the election in which a person gained a position from, or reelection in which the position was confirmed & MISC \\ \hline
        has effect & P1542 & mercury poisoning & effect of this item & MISC \\ \hline
        corrigendum / erratum & P2507 & Evolution in Mendelian Populations & published notice that corrects or amends a previous publication & MISC \\ \hline
        electoral district & P768 & Ohio's 8th congressional district & "electoral district this person is representing, or of the office that is being contested. Use as qualifier for ""position held"" (P39) or ""office contested"" (P541) or ""candidacy in election"" (P3602)" & MISC \\ \hline
        mascot & P822 & Scotty the Scottie Dog & mascot of an organization, e.g. a sports team or university & MISC \\ \hline
        facet of & P1269 & general relativity & topic of which this item is an aspect, item that offers a broader perspective on the same topic & MISC \\ \hline
        has cause & P828 & mercury & underlying cause, thing that ultimately resulted in this effect & MISC \\ \hline
        direction & P560 & north & qualifier to indicate the direction of the object relative to the subject item (for direction to the object, see P654) & MISC \\ \hline
        part of & P361 & head & "object of which the subject is a part (if this subject is already part of object A which is a part of object B, then please only make the subject part of object A). Inverse property of ""has part"" (P527, see also ""has parts of the class"" (P2670))." & MISC \\ \hline
        lifestyle & P1576 & vegetarianism & typical way of life of an individual, group, or culture & MISC \\ \hline
        writing system & P282 & English alphabet & alphabet, character set or other system of writing used by a language, supported by a typeface & MISC \\ \hline
        follows & P155 & Star Wars: Episode IV A New Hope & "immediately prior item in a series of which the subject is a part, preferably use as qualifier of P179 [if the subject has replaced the preceding item, e.g. political offices, use ""replaces"" (P1365)]" & MISC \\ \hline
        flag & P163 & flag of Slovakia & subject's flag & MISC \\ \hline
        part of the series & P179 & The Chronicles of Narnia & series which contains the subject & MISC \\ \hline
        means of locomotion & P3512 & bipedalism & method that the subject uses to move from one place to another & MISC \\ \hline
        color & P462 & black & color of subject & MISC \\ \hline
        constellation & P59 & Andromeda & the area of the celestial sphere of which the subject is a part (from a scientific standpoint, not an astrological one) & MISC \\ \hline
        medical examinations & P923 & medical radiography & examinations that might be used to diagnose and/or prognose the medical condition & MISC \\ \hline
        partially coincident with & P1382 & Interstate 76 & object that is partially part of, but not fully part of (P361), the subject & MISC \\ \hline
        catchphrase & P6251 & Did I do that? & commonly used phrase by which someone or something may be recognized & MISC \\ \hline
        stock exchange & P414 & New York Stock Exchange & exchange on which this company is traded & MISC \\ \hline
        motto text & P1451 & Un Dieu, un roy, une foy, une loy (French) & short motivation sentence associated to item & MISC \\ \hline
        level of description & P6224 & record group & position of the unit of description in the hierarchy of the fonds & MISC \\ \hline
        instrumentation & P870 & piano & combination of musical instruments employed in a composition or accompanying a (folk) dance & MISC \\ \hline
        footedness & P8006 & left-footedness & dominant foot or preferred stance of this person & MISC \\ \hline
        subclass of & P279 & fruit & next higher class or type; all instances of these items are instances of those items; this item is a class (subset) of that item. Not to be confused with P31 (instance of) & MISC \\ \hline
        domain of saint or deity & P2925 & sea & domain(s) which this saint or deity controls or protects & MISC \\ \hline
        charted in & P2291 & Billboard 200 & chart where the element reached a position & MISC \\ \hline
        radio format & P415 & rhythmic contemporary & describes the overall content broadcast on a radio station & MISC \\ \hline
        category contains & P4224 & architectural structure & category contains elements that are instances of this item & MISC \\ \hline
        theme music & P942 & St. Anger & the theme music/song used by the item & MISC \\ \hline
        sport & P641 & trail running & sport that the subject participates or participated in or is associated with & MISC \\ \hline
        mount & P3091 & Rocinante & creature ridden by the subject, for instance a horse & MISC \\ \hline
        notable work & P800 & Hamlet & notable scientific, artistic or literary work, or other work of significance among subject's works & MISC \\ \hline
        movement & P135 & Frankfurt School & literary, artistic, scientific or philosophical movement or scene associated with this person or work & MISC \\ \hline
        has pattern & P5422 & stripe & pattern, design, or motif intrinsic to, incorporated into, or applied to the surface of the subject & MISC \\ \hline
        history of topic & P2184 & history of Germany & "item about the historical development of an subject's topic, sample: ""history of Argentina"" for ""Argentina"". To list key events of the topic, use ""significant event"" (P793)" & MISC \\ \hline
        position played on team / speciality & P413 & centre & position or specialism of a player on a team & MISC \\ \hline
        basic form of government & P122 & unitary state & subject's government & MISC \\ \hline
        call sign & P2317 & Freedom 7 & short form identifier for a radio operator or broadcaster and (as flag signal) previous for watercrafts & MISC \\ \hline
        statistical unit & P2353 & country & member of a dataset & MISC \\ \hline
        cabinet & P5054 & Florida Cabinet & "qualifier for ""position held"" (P39) to indicate the cabinet to which belongs a minister" & MISC \\ \hline
        main subject & P921 & Rocco Granata & primary topic of a work (see also P180: depicts) & MISC \\ \hline
        Artsy gene & P2411 & cubism & generalization of artwork type, technique, material, genre, movement, etc. from artsy.net & MISC \\ \hline
        template has topic & P1423 & Syngnathiformes & topic related to template & MISC \\ \hline
        candidacy in election & P3602 & 2012 Finnish municipal elections & election where the subject is a candidate & MISC \\ \hline
        does not have part & P3113 & control tower & expected part that the item does not have (for qualities, use P6477) & MISC \\ \hline
        commemorates & P547 & Johann Sebastian Bach & what the place, monument, memorial, or holiday, commemorates & MISC \\ \hline
        alternate names & P4970 & hankies & qualifier for alternative name(s) given for a subject in a database entry & MISC \\ \hline
        iconographic symbol & P4185 & Keys of Heaven & identifying element typically depicted as accompanying or worn by this religious figure, hero, fictional or historical character & MISC \\ \hline
        cuisine & P2012 & Indian cuisine & type of food served by a restaurant or restaurant chain or national food culture & MISC \\ \hline
        possible medical findings & P5131 & mid-systolic click & possible medical findings of a medical condition & MISC \\ \hline
        parent taxon & P171 & Sus scrofa & closest parent taxon of the taxon in question & MISC \\ \hline
        presented in & P5072 & TED2010 & event at which a talk, film, paper, or poster was presented & MISC \\ \hline
        title & P1476 & Nature & published name of a work, such as a newspaper article, a literary work, piece of music, a website, or a performance work & MISC \\ \hline
        affiliation string & P6424 & Southampton University & qualifier to provide the published string form of affiliation attached to an author & MISC \\ \hline
        quotation or excerpt & P7081 & who would these fardels bear,/To grunt and sweat under a weary life,/But that the dread of something after death, The undiscover'd country, from whose bourn/No traveller returns, puzzles the will,/And makes us rather bear those ills we have/Than fly to others that we know naught of (English) & quotation or excerpt from this work. No quotation marks needed & MISC \\ \hline
        subject has role & P2868 & antineoplastic & "role/generic identity of the item (""subject""), also in the context of a statement. For the role of the value of the statement (""object""), use P3831 (""object has role""). For acting roles, use P453 (""character role""). For persons, use P39." & MISC \\ \hline
        item operated & P121 & transport infrastructure & equipment, installation or service operated by the subject & MISC \\ \hline
        sports competition competed at & P5249 & 2012 UEFA Champions League & edition of sports competitions at which the club or team that played a season competed at. Use this to link items for team seasons to items for specific seasons of competitions.Sample: 2012 ??? 13 FC Barcelona season ??? 13 UEFA Champions League & MISC \\ \hline
        literal translation & P2441 & first son (English) & direct or word-for-word translation of a name or phrase (qualifier for name, title, inscription, and quotation properties) & MISC \\ \hline
        from narrative universe & P1080 & Tolkien's legendarium & subject's fictional entity is in the object narrative. See also P1441 (present in work) and P1445 (fictional universe described in) & MISC \\ \hline
        seal description & P418 & Great Seal of the United States & links to the item for the subject's seal & MISC \\ \hline
        anthem & P85 & State Anthem of the Soviet Union & subject's official anthem & MISC \\ \hline
        taxon name & P225 & Panthera leo & correct scientific name of a taxon (according to the reference given) & MISC \\ \hline
        wears & P3828 & engagement announcement dress of Catherine Middleton & clothing or accessory worn on subject's body & MISC \\ \hline
        studies & P2578 & Ancient Egypt & the object that an academic field studies; distinct from field of work (P101), which is used for human, organization, etc. & MISC \\ \hline
        business model & P7936 & free-to-play & business model a business enterprise or creative work operates under & MISC \\ \hline
        social classification & P3716 & commoner & social class as recognized in traditional or state law & MISC \\ \hline
        record held & P1000 & men's pole vault world record & notable record achieved by a person or entity, include qualifiers for dates held & MISC \\ \hline
        named after & P138 & Camembert & "entity or event that inspired the subject's name, or namesake (in at least one language). Qualifier ""applies to name"" (P5168) can be used to indicate which one" & MISC \\ \hline
        general classification of race participants & P2321 & Nacer Bouhanni & classification of race participants & MISC \\ \hline
        tracklist & P658 & Wanna Be Startin' Somethin' & audio tracks contained in this release & MISC \\ \hline
        nickname & P1449 & The Golden State & informal name (for a pseudonym use P742) & MISC \\ \hline
        shooting handedness & P423 & left-handed shot & whether the hockey player passes or shoots left- or right-handed & MISC \\ \hline
        significant event & P793 & Battle of Dennewitz & significant or notable events associated with the subject & MISC \\ \hline
        followed by & P156 & April & "immediately following item in a series of which the subject is a part, preferably use as qualifier of P179 [if the subject has been replaced, e.g. political offices, use ""replaced by"" (P1366)]" & MISC \\ \hline
        manner of inhumane treatment & P7160 & sleep deprivation & manner of torture and other cruel, inhumane or degrading treatment or punishments as covered by the UN Convention experienced by the subject & MISC \\ \hline
        possessed by spirit & P4292 & Pazuzu & item which is spiritually possessing this item & MISC \\ \hline
        fandom & P8693 & A.I Troops & fan group name of a celebrity, musical group, or an artist & MISC \\ \hline
        input method & P479 & computer keyboard & input method or device used to interact with a software product & MISC \\ \hline
        damaged & P3081 & Upper Basilica of San Francesco d'Assisi & physical items damaged by this event & MISC \\ \hline
        plea & P1437 & guilt & whether a person pleaded guilty, not guilty, etc. & MISC \\ \hline
        derivative work & P4969 & MX Linux & new work of art (film, book, software, etc.) derived from major part of this work & MISC \\ \hline
        dataset distribution & P2702 & Art \& Architecture Thesaurus LOD Dataset & particular manner of distribution of a data set (database or file) that is publicly available & MISC \\ \hline
        real estate developer & P6237 & Strabag Real Estate & person or organization responsible for building this item & MISC \\ \hline
        product or material produced & P1056 & uranium & material or product produced by a government agency, business, industry, facility, or process & MISC \\ \hline
        contributed to creative work & P3919 & Dictionary of National Biography & "person is cited as contributing to some creative or published work or series (qualify with ""subject has role"", P2868)" & MISC \\ \hline
        military casualty classification & P1347 & killed in action & allowed values:  killed in action (Q210392), missing in action (Q2344557), died of wounds (Q16861372), prisoner of war (Q179637), killed in flight accident (Q16861407), others used in military casualty classification & MISC \\ \hline
        separated from & P807 & Presbyterian Church in the United States & subject was founded or started by separating from identified object & MISC \\ \hline
        results & P2501 & general classification of the 2015 Coupe Sels & results of a competition such as sports or elections & MISC \\ \hline
        ritual object & P8706 & corpse powder & ceremonial or ritual objects associated with, and used as part of, rites and rituals practiced in everyday life and in rarer cultic and communal rites & MISC \\ \hline
        edition or translation of & P629 & Pride and Prejudice & is an edition or translation of this entity & MISC \\ \hline
        Catholic rite & P3501 & Roman Rite & Christian liturgical rite associated with this item & MISC \\ \hline
        academic minor & P811 & political science & minor someone studied at college/university & MISC \\ \hline
        intangible cultural heritage status & P3259 & inventory of intangible cultural heritage in France & status of an item that is designated as intangible heritage & MISC \\ \hline
        opposite of & P461 & peace & item that is the opposite of this item & MISC \\ \hline
        reward & P4444 & travel insurance & reward, bonus, or prize received as part of a membership or loyalty program & MISC \\ \hline
        award received & P166 & Theodor Haecker Price & award or recognition received by a person, organisation or creative work & MISC \\ \hline
        legal form & P1454 & GmbH \& Co. KG & legal form of an entity & MISC \\ \hline
        Bharati Braille & P9021 & braille script & transcription of Indic scripts in a national standard Braille script & MISC \\ \hline
        vehicle normally used & P3438 & popemobile & vehicle the subject normally uses & MISC \\ \hline
        coat of arms & P237 & Coat of arms of Liechtenstein & subject's coat of arms & MISC \\ \hline
        convicted of & P1399 & murder & crime a person was convicted of & MISC \\ \hline
        made from material & P186 & chocolate liquor & material the subject or the object is made of or derived from & MISC \\ \hline
        competition class & P2094 & Group R & official classification by a regulating body under which the subject (events, teams, participants, or equipment) qualifies for inclusion & MISC \\ \hline
        shape & P1419 & pyramid & shape of an object & MISC \\ \hline
        academic thesis & P1026 & Die Rechtsform der Kartelle mit einer als selbständige Handels-Gesellschaft organisierten Verkaufsstelle (Doppel-Gesellschaft) unter Berücksichtigung ihrer Steuerleistungspflicht & thesis or dissertation written for a degree & MISC \\ \hline
        audio system & P7501 & bell & audio system hardware used in the item & MISC \\ \hline
        first appearance & P4584 & A Study in Scarlet & work in which a fictional/mythical character or entity first appeared & MISC \\ \hline
        last words & P3909 & I want nothing but death. & last words attributed to a person before their death & MISC \\ \hline
        strand orientation & P2548 & software & orientation of gene on double stranded DNA molecule & MISC \\ \hline
        female form of label & P2521 & autora & female form of name or title & MISC \\ \hline
        penalty & P1596 & capital punishment & penalty imposed by an authority & MISC \\ \hline
        handedness & P552 & right-handedness & handedness of the person & MISC \\ \hline
        Google Play developer slug & P8939 & Facebook & human-readable identifier for a developer on the Google Play Store & MISC \\ \hline
        instrument & P1303 & drum & musical instrument that a person plays or teaches or used in a music occupation & MISC \\ \hline
        index case of & P1677 & Ebola virus disease in the United States & primary case, patient zero: initial patient in the population of an epidemiological investigation & MISC \\ \hline
        reward program & P4446 & Chase Ultimate Rewards & reward program associated with the item & MISC \\ \hline
        charge & P1595 & seditious libel & offence with which someone is charged, at a trial & MISC \\ \hline
        had as last meal & P3902 & ice cream & components of the last meal had by a person before death & MISC \\ \hline
        relevant qualification & P4968 & Project Management Professional & practitioners of this industry get this degree, licence or certification after specialist education, apprenticeship, or professional review. This includes qualifications that one needs to obtain in order to join the industry or qualifications that one obtains after a certain level of experience in the industry in order to progress further in their career. & MISC \\ \hline
        for work & P1686 & Little Life & qualifier of award received (P166) to specify the work that an award was given to the creator for & MISC \\ \hline
        interested in & P2650 & The Holocaust & item of special or vested interest to this person or organisation & MISC \\ \hline
        health specialty & P1995 & ophthalmology & main specialty that diagnoses, prevent human illness, injury and other physical and mental impairments & MISC \\ \hline
        appears in the form of & P4675 & bull & this fictional or mythical entity takes the form of that entity & MISC \\ \hline
        vessel class & P289 & Concordia-class cruise ship & series of vessels built to the same design of which this vessel is a member & MISC \\ \hline
        medical condition treated & P2175 & non-small-cell lung carcinoma & disease that this pharmaceutical drug, procedure, or therapy is used to treat & MISC \\ \hline
        sports discipline competed in & P2416 & marathon & discipline an athlete competed in within a sport & MISC \\ \hline
        madhhab & P9929 & Shafi`i & Islamic school of thought within Fiqh & MISC \\ \hline
        cause of death & P509 & nitric acid poisoning & underlying or immediate cause of death.  Underlying cause (e.g. car accident, stomach cancer) preferred.  Use 'manner of death' (P1196) for broadest category, e.g. natural causes, accident, homicide, suicide & MISC \\
\end{longtable}

\end{appendices}
